# Supplementary material for: Sensing and Communication with Quantum Microwaves
Source: arXiv:2310.04838 source file (2023-10-07)
Supplement: Supplementary file 1 [file CRB.tex]

%!TEX root = ../dissertation.tex

\chapter{Proof of the Cramér-Rao inequality}
\label{appendix:CRB}

\textbf{NOTE (26 May 2023): do I really need this appendix? If so, needs rewriting. I think it can be left for the defense, as extra slide (already have it in that format from the Bilbao seminar I gave).}

Sketch of proof of Cramér-Rao inequality (I)
%%%%This slide should be an extra slide for questions
Good reference is\foonote{G. Casella and R. Berger, Statistical Inference (2002)}.\\
Consider Cauchy-Schwarz inequality:
$$|\langle \bm{X}, \bm{Y}\rangle |^2 \leq \langle \bm{X}, \bm{X}\rangle   \langle \bm{Y}, \bm{Y}\rangle $$
where $\langle \cdot, \cdot \rangle$ is an inner product.

\begin{itemize}
\item Need an inner product space: choose expectation $E$ as inner product. Assume integrability.
\item Then $|E[\bm{X}\bm{Y}]|^2 \leq E[\bm{X}\bm{X}]E[\bm{Y}\bm{Y}]$
\end{itemize}
Use definition of covariance:
$$\text{Cov}(\bm{X}, \bm{Y}) = E[(\bm{X}-E[\bm{X}])(\bm{Y}-E[\bm{Y}])]$$
And of variance:
$$\text{Var}(\bm{X}) = E[(\bm{X}-E[\bm{X}])^2]$$

Sketch of proof of Cramér-Rao inequality (II)
%%%%This slide should be an extra slide for questions
So the C-S inequality translates to 
$$ |\text{Cov}(\bm{X}, \bm{Y})|^2 \leq \text{Var}(\bm{X}) \text{Var}(\bm{Y})$$
Or, rearranging:
$$ \text{Var}(\bm{X})  \geq \frac{|\text{Cov}(\bm{X}, \bm{Y})|^2}{\text{Var}(\bm{Y})}$$
Now,
\begin{itemize}
\item Choose $\bm{X}$ to be the estimator $\hat{\lambda}$.
\item Choose  $\bm{Y}$ to be $\partial_\lambda \ln p(\bm{x}|\lambda)$ .
\item Where $\bm{x} = (x_1, x_2, \ldots, x_M)$.
\item Do some algebra and be careful. 
\end{itemize}
